# Supplementary material for: Cross-Domain Correlation Distillation for Unsupervised Domain Adaptation in Nighttime Semantic Segmentation
Source: arXiv:2205.00858 source file (2022-05-02)
Supplement: Supplementary file 1 [file supplement.tex]

\begin{table}
\centering
\setlength{\tabcolsep}{1mm}{ %< auto-adjusts font size to fill line
\setlength{\abovecaptionskip}{1pt}
\caption{
Additional ablation studies of our proposed method on Dark Zurich-test set.
} % \caption
\setlength{\belowcaptionskip}{1pt}
\label{tab:supplement}
\begin{tabular}{@{}lc@{}}
\toprule
Method & mIoU \\
\midrule
RefineNet &  28.5\\
\midrule
w/o project head and $L_{JS}$ in CDC & 41.6\\
w/o illuminance and inherent correlation in CDC &  43.8\\
\midrule
\textbf{Ours} & 47.5\\
\bottomrule
\end{tabular}
} %< \resizebox
\end{table}
