# Supplementary material for: Cross-Domain Correlation Distillation for Unsupervised Domain Adaptation in Nighttime Semantic Segmentation
Source: arXiv:2205.00858 source file (2022-05-02)
Supplement: Supplementary file 3 [file supplement_bdd.tex]

\begin{figure*}
\begin{center}
\includegraphics[width=\linewidth]{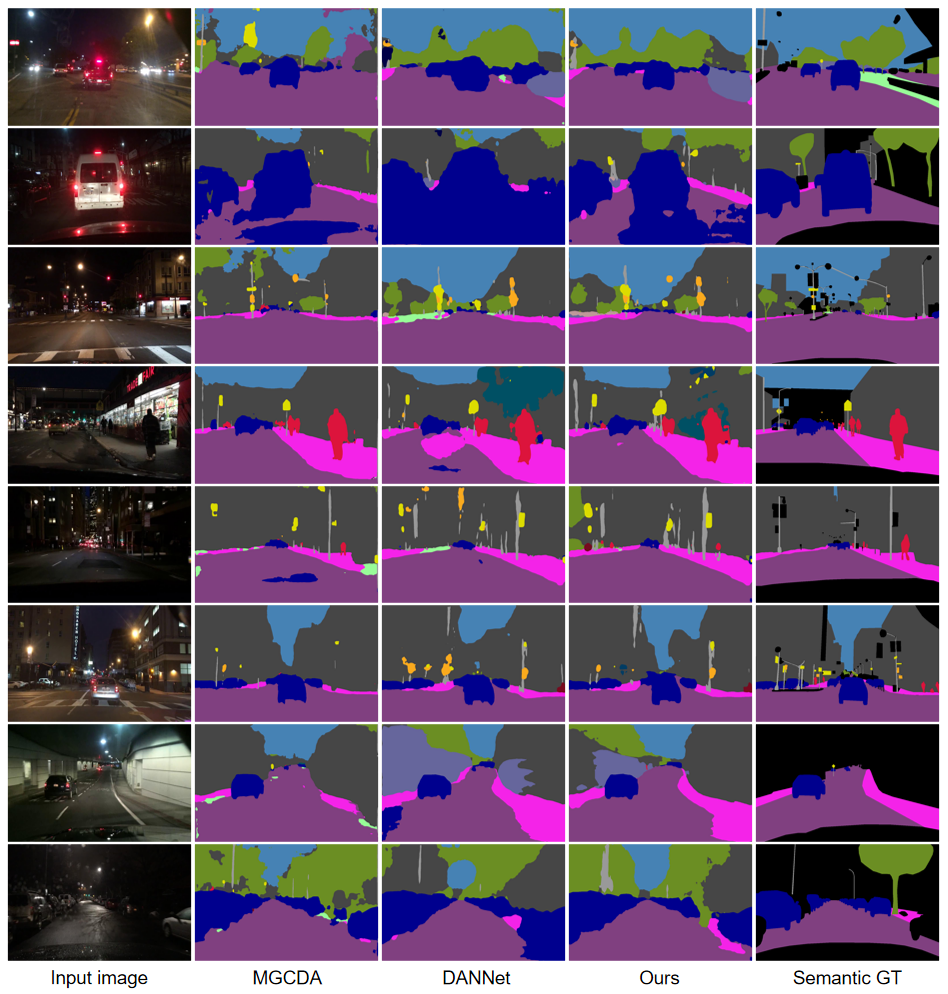}
\hfill
\end{center}
\setlength{\abovecaptionskip}{1pt}
\caption{
The qualitative comparison between our approach and some existing state-of-the-art methods on the BDD100K-night set.
}
\setlength{\belowcaptionskip}{1pt}
\label{fig:supplement_bdd}
\end{figure*}
